# Supplementary material for: MuLTI: Efficient Video-and-Language Understanding with Text-Guided MultiWay-Sampler and Multiple Choice Modeling
Source: arXiv:2303.05707 source file (2024-03-01)
Supplement: Supplementary file 1 [file 6-appendix.tex]

\clearpage
\appendix 
\onecolumn
\section*{A. Appendix}
\subsection*{A.1. Examples for Multi-Label Classification}
\begin{multicols}{2} 
%We cannot make the Chinese multi-label dataset publicly available for privacy reasons. 
In the Appendix, we show some typical examples of multi-label classification. Each example consists of four parts: video sparse frames, text, OCR transcripts and predicted labels. In each example, \textbf{Text} refers to the description text of the video, \textbf{OCR} is the combination of the OCR transcripts for each sparse frame in the video, and \textbf{Pred} is the predicted labels of MuLTI. The \textbf{...} indicates that the OCR transcripts are truncated due to limited space. The threshold value of the predicted label is 0.5. Red predicted labels are the wrong predicted labels.
\end{multicols}
\begin{figure*}[ht]
\centering
\includegraphics[width=0.85\textwidth]{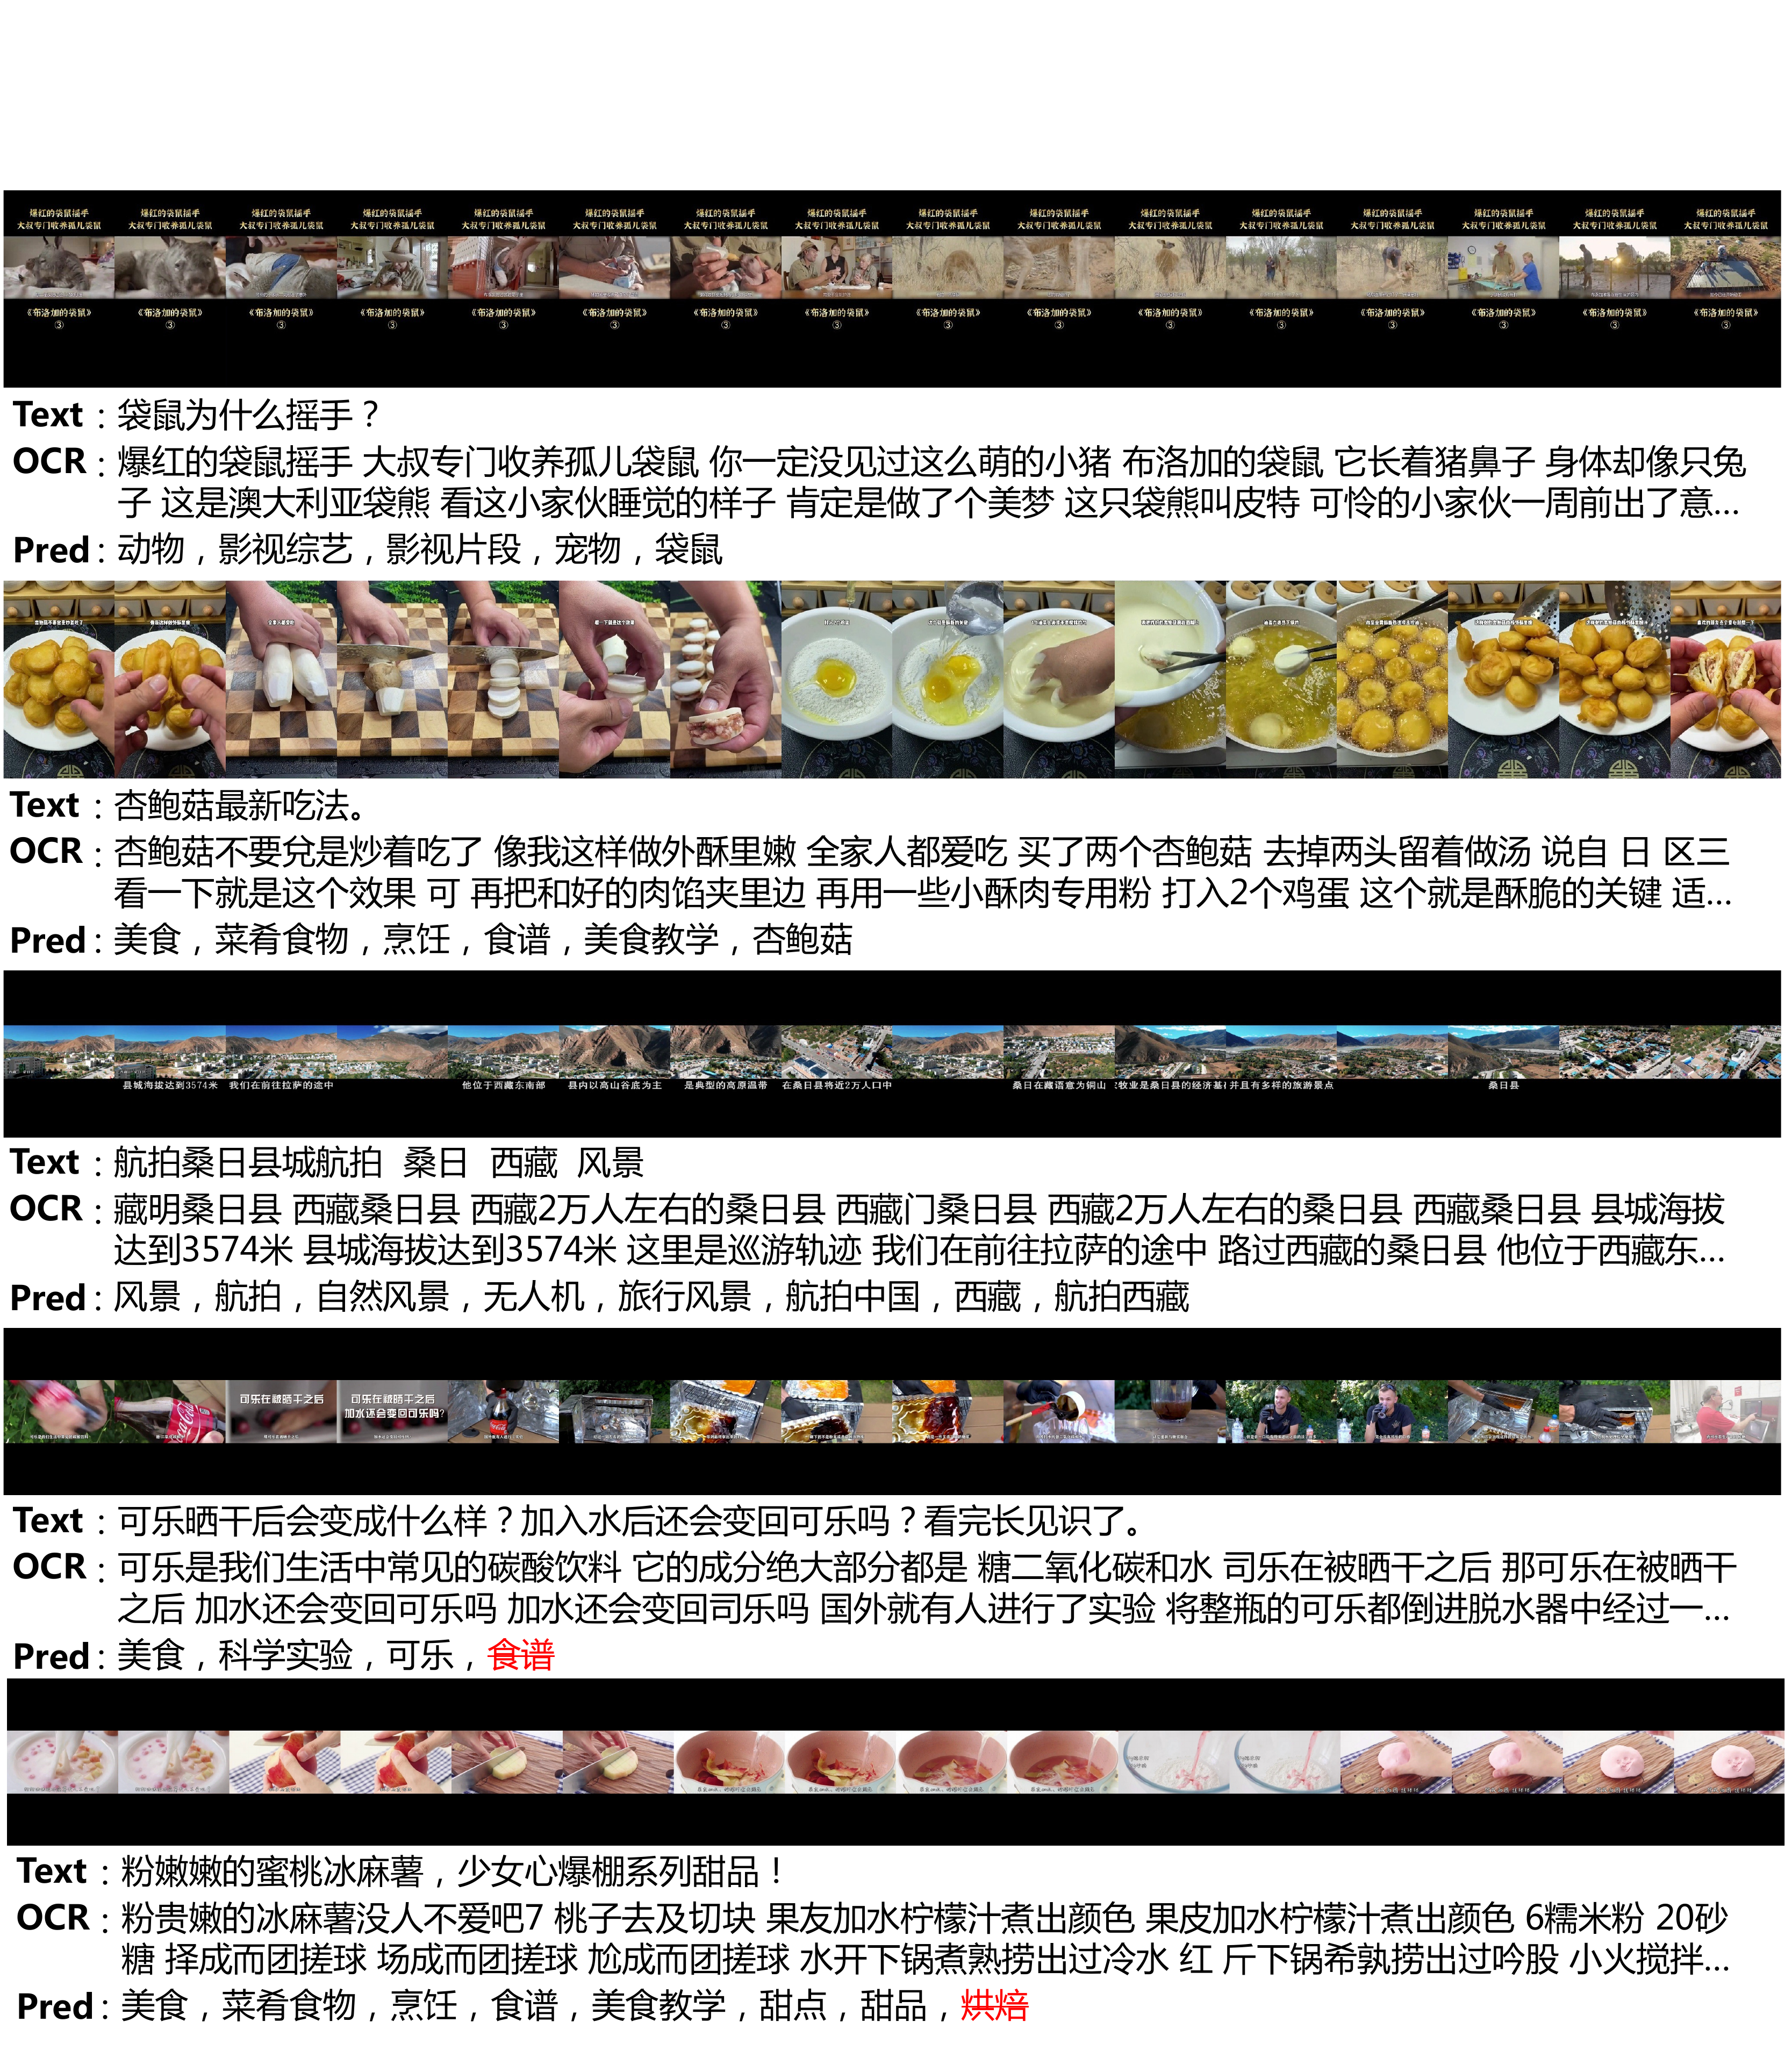}
% \vspace{1ex}
\caption{
Examples of multi-label classification. \textbf{Text} refers to the description text of the video. \textbf{OCR} refers to the combination of OCR transcripts of each sparse frame in the video. \textbf{Pred} refers to the prediction results of MuLTI. The \textbf{...} indicates that the OCR transcripts are truncated due to limited space. The threshold value of the predicted label is 0.5. Red predicted labels are the wrong predicted labels.
}
% \vspace{1ex}
\label{fig:appendix}
\end{figure*}
